# Supplementary material for: Plasmon Excitations Across the Charge-Density-Wave Transition in Single-Layer TiSe$_2$
Source: arXiv:2307.11370 ancillary file (2024-05-22)
Supplement: Supplementary file 1 [file tise2_SI.pdf]

# Supporting information for: Plasmon Excitations Across the Charge-Density-Wave Transition in Single-Layer $TiSe_2$

Zahra Torbatian† and Dino Novko*,‡,¶

†*School of Nano Science, Institute for Research in Fundamental Sciences (IPM), 19395-5531 Tehran, Iran*

‡*Centre for Advanced Laser Techniques, Institute of Physics, 10000 Zagreb, Croatia*

¶*Donostia International Physics Center (DIPC), 20018 Donostia-San Sebastián, Spain*

E-mail: dino.novko@gmail.com

## S1 Theory and computational details

All the calculations were performed within the framework of the density functional theory (DFT) within the QUANTUM ESPRESSO package [S1]. Optimized norm-conserving Vanderbilt pseudopotentials [S2] were used with the PBE exchange-correlation functional [S3] from the PseudoDojo library [S4]. The plane wave energy cutoff was fixed to 80 Ry. The 2D layers are modeled in periodic cells with 20 Å vacuum in the direction normal to the layer to reduce the interaction between the periodic images. The convergence criterion for energy is set to $10^{-8}$ eV and the atomic positions are relaxed until the Hellmann-Feynman forces are less than $10^{-4}$ eV/Å. A lattice parameter of $a = 3.537$ Å is obtained with the PBE functional. To obtain the ground state charge density the 2D Brillouin

zone is sampled with $48 \times 48 \times 1$ k-point mesh. The Fermi-Dirac smearing functions were used with the electronic temperatures $T_{\mathrm{scf}}$ ranging from 100 K to 1600 K. To accurately determine the electron-phonon coupling (EPC), we employed the Wannier interpolation technique [S5], which has been implemented in the EPW code [S6]. To do so, the electronic structure, dynamical matrices, and electron-phonon matrix elements were obtained from DFT and density functional perturbation theory (DFPT) [S7] calculations, and they were used as the initial data for Wannier interpolation with the maximally-localized Wannier functions. Initial DFPT phonon calculations were done on corse grids of $\mathbf{k} = 24 \times 24 \times 1$ and $\mathbf{q} = 6 \times 6 \times 1$ for the $1 \times 1$ structure, while on $\mathbf{k} = 12 \times 12 \times 1$ and $\mathbf{q} = 3 \times 3 \times 1$ for the distorted $2 \times 2$ CDW structure, as well as for various $T_{\mathrm{scf}}$ mentioned above. The soft acoustic phonon mode goes to zero at $T_{\mathrm{scf}} = 1105$ K, and below this temperature we need to consider the $2 \times 2$ CDW structure [S8].

In the following, we briefly describe a methodology for the calculation of optical absorption in the long-wavelength limit ($\mathbf{q} \approx 0$) by making use of the current-current response function $\Pi_\mu(\mathbf{q}, \omega)$ calculated within DFT, where the electromagnetic interaction is mediated by the free-photon propagator. For a more thorough description of the method, we refer reader to our previous work [S9]. Note that the atomic units (a.u.) are used throughout this work.

In this study, the electron excitation spectral function is a key quantity that is defined as $A(\mathbf{q}, \omega) = -4\hbar \mathrm{Im}\, \Pi_\mu(\mathbf{q}, \omega)/\omega$, while the optical conductivity is $\sigma_\mu(\omega) = -i\Pi^0_\mu(\mathbf{q} = 0, \omega)/\omega$, where $\Pi^0_\mu(\mathbf{q}, \omega)$ is a bare, while $\Pi_\mu(\mathbf{q}, \omega)$ is a fully screened current-current correlation function. In particular, optical excitations can be written in terms of the intraband ($n = m$) and interband ($n \neq m$) contributions, i.e., $\Pi^0_\mu = \Pi^{0,\mathrm{intra}}_\mu + \Pi^{0,\mathrm{inter}}_\mu$. The bare current-current correlation function $\Pi^0_\mu$ is screened with Coulomb interaction by the following Dyson equation $\Pi_\mu = \Pi^0_\mu + \Pi^0_\mu \otimes D \otimes \Pi_\mu$ (where $D$ is the photon propagator). To investigate the effects of phonons on the plasmon dispersion, we implement the formalism presented in Ref. S10, where the electron-phonon scattering mechanism is considered in the intraband channel. Note that the present method ensures that the Coulomb (or photon-electron) interaction between the neighbouring cells in the perpendicular direction is properly truncated [S9], which ensures the screening and Coulomb interaction are truly quasi-2D.

The non-interacting interband current-current response tensor in the optical limit (when $\mathbf{q} \approx 0$), is built from ground-state Kohn-Sham eigenvalues $E_n(\mathbf{k})$ and the current vertices, $J^{\mu}_{nm\mathbf{k}}$:

$$\Pi^{0,\mathrm{inter}}_{\mu}(\omega) = \frac{2}{V}\sum_{\mathbf{k},n\neq m}\left|J^{\mu}_{nm\mathbf{k}}\right|^2 \frac{\hbar\omega}{E_n(\mathbf{k})-E_m(\mathbf{k})}\frac{f_n(\mathbf{k})-f_m(\mathbf{k})}{\hbar\omega+i\eta+E_n(\mathbf{k})-E_m(\mathbf{k})}, \tag{S1}$$

where $f_n(\mathbf{k})$ is the Fermi-Dirac distribution function at temperature $T$, $\mu$ are the polarization directions, $V$ is the normalized volume, and $\eta$ is the interband damping parameter. Further, the summation over $\mathbf{k}$ wavevectors is carried out on $160 \times 160 \times 1$ and $80 \times 80 \times 1$ grids for the normal $1 \times 1$ and CDW $2 \times 2$ phases of $1T$-$TiSe_2$, respectively, while the $n$ and $m$ band indices go over 40 electronic bands.

The corresponding intraband contribution of current-current response tensor can be written as the following[S10]:

$$\Pi^{0,\mathrm{intra}}_{\mu}(\omega) = \frac{2}{V}\frac{\omega}{\omega[1+\lambda_{\mathrm{ep}}(\omega)]+i/\tau_{\mathrm{ep}}(\omega)}\sum_{\mathbf{k},n}\frac{\partial f_{nk}}{\partial E_{n\mathbf{k}}}|J^{\mu}_{nn\mathbf{k}}|^2. \tag{S2}$$

The effects of the EPC is considered through the temperature-dependent dynamical scattering time and the energy renormalization functions, i.e., $\tau_{\mathrm{ep}}(\omega)$ and $\lambda_{\mathrm{e}}(\omega)$, respectively. The temperature-dependent dynamical scattering time is given by [S11]

$$\hbar/\tau_{\mathrm{ep}}(\omega) = \frac{\pi\hbar}{\omega}\int d\Omega\alpha^2F(\Omega)\Big[2\omega\coth\frac{\Omega}{2k_BT} - (\omega+\Omega)\coth\frac{\omega+\Omega}{2k_BT} + (\omega-\Omega)\coth\frac{\omega-\Omega}{2k_BT}\Big] \tag{S3}$$

where $k_B$ is the Boltzmann constant and $\alpha^2F(\Omega)$ is the Eliashberg spectral function [S10]

$$\alpha^2F(\omega) = \frac{1}{2\pi N(E_F)}\sum_{\mathbf{q}\nu}\delta(\omega-\omega_{\mathbf{q}\nu})\frac{\gamma_{\mathbf{q}\nu}}{\hbar\omega_{\mathbf{q}\nu}}, \tag{S4}$$

where $N(E_F)$ is the density of states at the Fermi level, while $\omega_{\mathbf{q}\nu}$ and $\gamma_{\mathbf{q}\nu}$ are the frequency and linewidth for the phonon mode $\nu$ at wavevector $\mathbf{q}$. Finally, the dynamical energy renormalization parameter $\lambda_{\mathrm{ep}}(\omega)$ is obtained by performing the Kramers-Kronig transformation of $1/\tau_{\mathrm{ep}}(\omega)$.

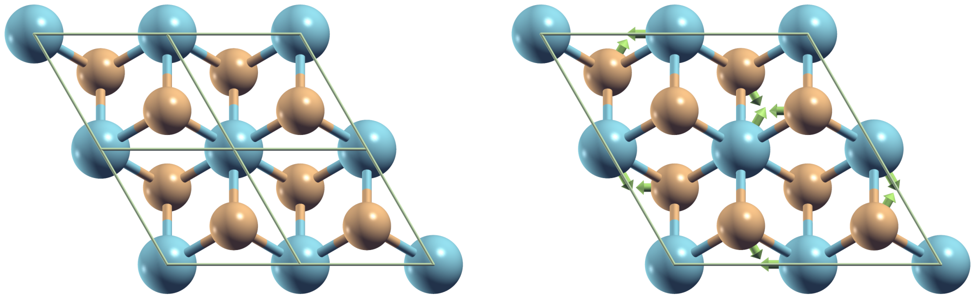

Figure S1: Unit cell of the $1 \times 1$ undistorted structure stable for $T \geq T_{\mathrm{CDW}}$ (left panel), and the $2 \times 2$ phase with periodic lattice distortions shown with green arrows stable for $T < T_{\mathrm{CDW}}$ (right panel).

The phonon properties (i.e., phonon energies and electron-phonon matrix elements), needed for calculating $\alpha^2 F(\omega)$ are obtained within the EPW code [S6]. The calculations of the EPC constants and Eliashberg function are performed on dense $\mathbf{k} = 600 \times 600 \times 1$ and $\mathbf{q} = 120 \times 120 \times 1$ grids for the undistorted normal phase, while on $\mathbf{k} = 300 \times 300 \times 1$ and $\mathbf{q} = 60 \times 60 \times 1$ grids for the $2 \times 2$ distorted CDW phase, which ensures the numerical convergence of the results presented in this work.

Depending on the (electron) temperature we calculate the EPC and optical properties as described above either for the $1 \times 1$ unit cell of $TiSe_2$ or for the $2 \times 2$ CDW structure with periodic lattice distortions (PLD). See Fig. S1. Namely, for $T < T_{\mathrm{CDW}}$ (where we get $T_{\mathrm{CDW}} = 1105\,\mathrm{K}$ for the harmonic DFPT calculations with PBE [S8]) we perform the above calculations for the $2 \times 2$ structures with PLDs. Note that for each temperature below $T_{\mathrm{CDW}}$ the PLDs are different (see Fig. S2), and calculations need to be done on separate structures. And for $T > T_{\mathrm{CDW}}$ we perform all of the calculations for the undistorted $1 \times 1$ structure. Note the good agreement between the PBE results for PLDs and experimental results of XRD study [S12].

A crucial thing to emphasize for the calculation of $1/\tau_{\mathrm{ep}}$ across the CDW transition is that for the input temperatures of Eq. (S3) we have used the room temperature $T = 300\,\mathrm{K}$ instead of the high temperatures obtained with harmonic PBE calculations near $T_{\mathrm{CDW}}$. First, the calculation of phonon energies were done by using the actual temperatures necessary to obtain the CDW transition with PBE functional, i.e., phonons of $1 \times 1$ structure for $T > T_{\mathrm{CDW}}$ were calculated for $T > 1105\,\mathrm{K}$, while

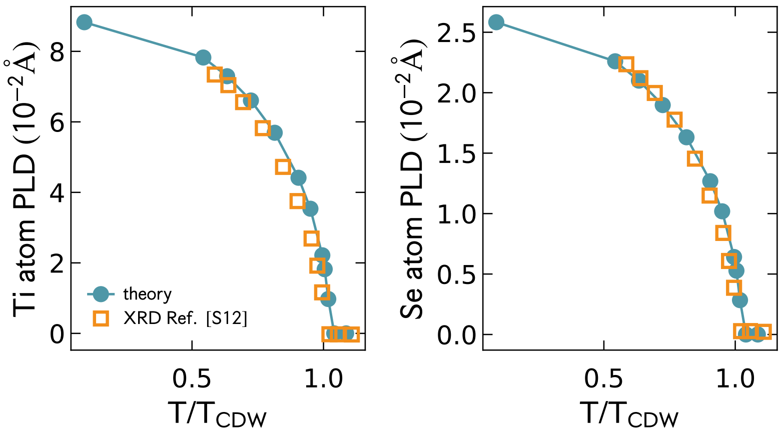


Figure S2: Periodic lattice distortions (PLD) for Ti and Se atoms as a function of electron temperature. For each of these new PLDs we perform new set of calculations of EPC and optical properties. Distortions of these atoms lead to the opening of the CDW gap close to the Fermi level. Our results of PLDs are in a good agreement with XRD study [S12].

phonons of $2 \times 2$ structure were obtained for $T < 1105$ K. However, when we calculate $\alpha^2 F(\omega)$ and $1/\tau_{ep}$ we do not shift the chemical potential in accordance to the high temperatures obtained with PBE, but we keep it at $T = 300$ K. Also, the temperatures entering Eq. (S3) are kept at $T = 300$ K. Namely, since we use harmonic PBE approach, we only include the electron entropy of the system and therefore we highly overestimate the transition temperature, i.e., $T_{\rm CDW}^{\rm PBE} \gg T_{\rm CDW}^{\rm exp}$. Thus the modifications of the chemical potential (due to conservation of particle number) are not realistic within PBE and are exaggerated. This could be corrected by employing the fully anharmonic approach and get the right transition temperature, but that could be numerically heavy since on top of the phonon calculations we need to do also the EPC calculations and simulations of plasmon dynamics. Instead of that, we simply use $T = 300$ K for calculations of $\alpha^2 F(\omega)$ and $1/\tau_{ep}$, which is close to temperature regime of $T_{\rm CDW}^{\rm exp}$. This provides the result of $1/\tau_{ep}$ that is in a close agreement with experiments, as indicated in the main text (see also blue dots in Fig. S3). On the other hand, if we use the high temperatures $T_{\rm scf}^{\rm PBE}$ and the corresponding exaggerated chemical potential shifts, we get the exaggerated values of $1/\tau_{ep}$ near $T_{\rm CDW}^{\rm PBE} = 1105$ K (see the orange dots in Fig. S3). Even more exaggerated values of $1/\tau_{ep}$ are obtained when the high temperatures $T_{\rm scf}^{\rm PBE}$ are used also in Eq. (S3) (see the red empty dots in Fig. S3).

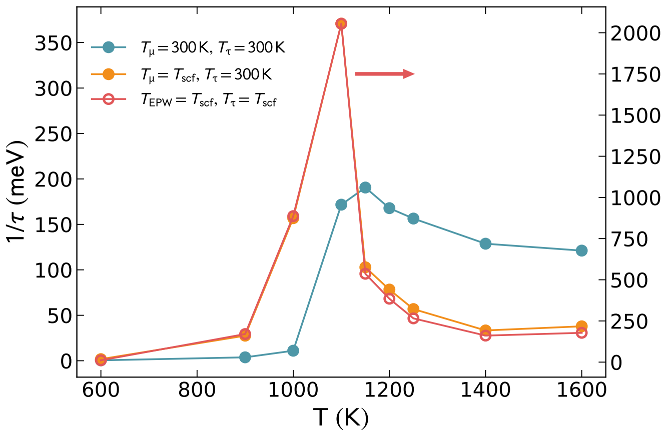


Figure S3: Electron-hole scattering rate due to EPC $1/\tau_{ep}$ when the chemical potential and Eq. (S3) are calculated at $T = 300$ K (blue dots), when the chemical potential is shifted according to the high temperatures near $T_{CDW}^{PBE} = 1105$ K, while temperature in Eq. (S3) is fixed at $T = 300$ K (orange dots), and when both the chemical potential and Eq. (S3) are calculated with high temperatures $T_{scf}^{PBE}$ obtained in PBE harmonic calculations of CDW transition.

We note that the calculations of current-current response functions Eqs. (S1) and (S2) are also calculated with Fermi-Dirac occupations (and chemical potentials) at $T = 300$ K, while Kohn-Sham energies, wavefunctions, and current vertices entering these equations are calculated for high temperatures $T_{scf}^{PBE}$ obtained in PBE calculations (and the corresponding structures). However, in this case it makes no difference in taking high temperatures $T_{scf}^{PBE}$ instead of $T = 300$ K.

The final results of the electron excitation spectra that include all the above essential ingredients are presented in Fig. S4 for low-temperature, intermediate, and high-temperature phases of $TiSe_2$. It is evident that the excitation spectra experience drastic modifications across the CDW transition, and show the strong interaction between the CDW electronic excitations and 2D plasmon mode.

# S2 Optical conductivity of the CDW phase - theory vs. experiments

In Fig. S5 we show the results for the real part of optical conductivity as obtained with Eqs. (S1) and (S2). The results are shown for the $2 \times 2$ CDW phase at $T = 100$ K, and for different interband

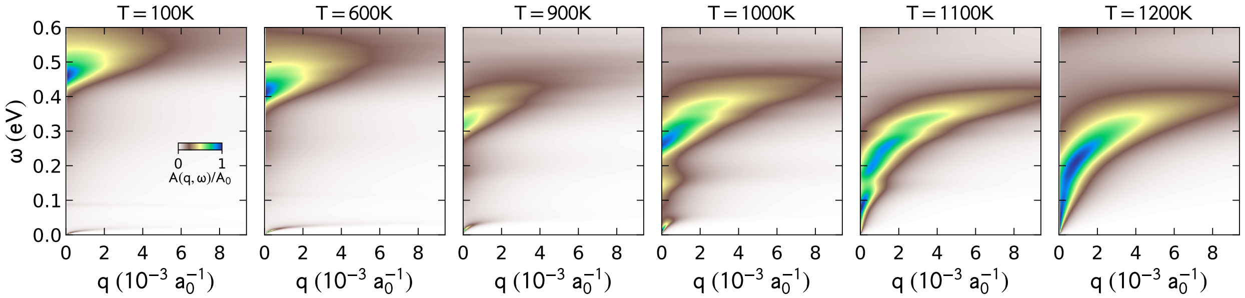


Figure S4: Low-energy electron excitation spectra $A(q,\omega)$ of single-layer $TiSe_2$ for several temperatures below and above $T_{CDW}$. The low-temperature regime is dominated by the interband excitations between 0.4 eV and 0.5 eV. In the high-temperature phase, the dominant excitation mode is the 2D plasmon with $\sqrt{q}$ dispersion. In the intermediate temperature range, we see the lowering of the interband CDW excitations and strengthening of the 2D plasmon with temperature increase, which around $T_{CDW}$ results in the hybrid CDW-plasmon mode.

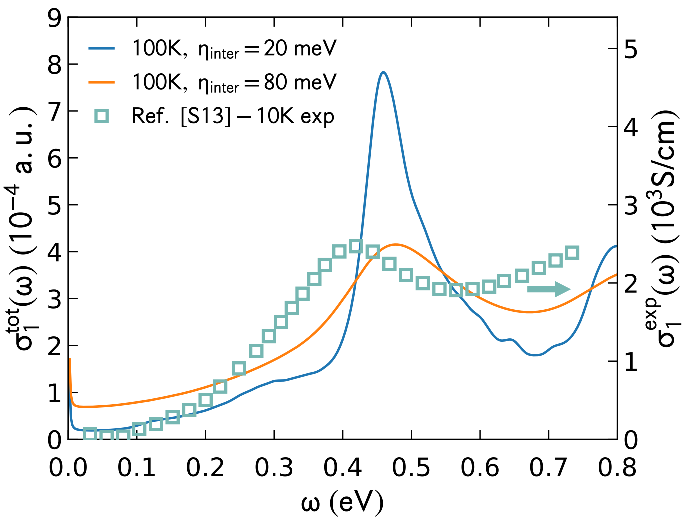


Figure S5: The real part of optical conductivity for the $2 \times 2$ CDW phase at $T = 100$ K, and for different interband damping parameters $\eta_{inter}$. The results obtained with the infrared optical spectroscopy at $T = 10$ K are shown for comparison [S13].

damping parameters $\eta_{inter}$ entering Eq. (S1). Our calculations are compared with the infrared optical measurments at $T = 10$ K [S13]. The agreement is obtained for larger $\eta_{inter}$, which confirms that the strong scatterings are active in the interband channel. Note that the calculated position of the high-energy peak is shifted by 44 meV compared to the experiment, which is reasonable considering that we do not include energy renormalizations of electron-hole states in the interband channel

Eq. (S1) (i.e., the interband gap) [S14].

Further, in Fig. S6 we show the optical conductivity for the $2 \times 2$ CDW phase at $T = 1000\,\mathrm{K}$, i.e., slightly below the $T_{\mathrm{CDW}}$, and for small ($\eta_{\mathrm{inter}} = 20\,\mathrm{meV}$) and large ($\eta_{\mathrm{inter}} = 80\,\mathrm{meV}$) values of interband excitation damping. When the large damping parameter $\eta_{\mathrm{inter}}$ is considered, the optical conductivity only shows the high-energy peak. This result explains why the optical conductivity measurements in Ref. S13 report only one CDW-related (i.e., high-energy) excitation in the low-temperature $2 \times 2$ phase of $TiSe_2$. On the other hand, our results reported here, as well as RIXS results from Ref. S15, show that there are two distinguished excitations peak related to the CDW interband transitions.

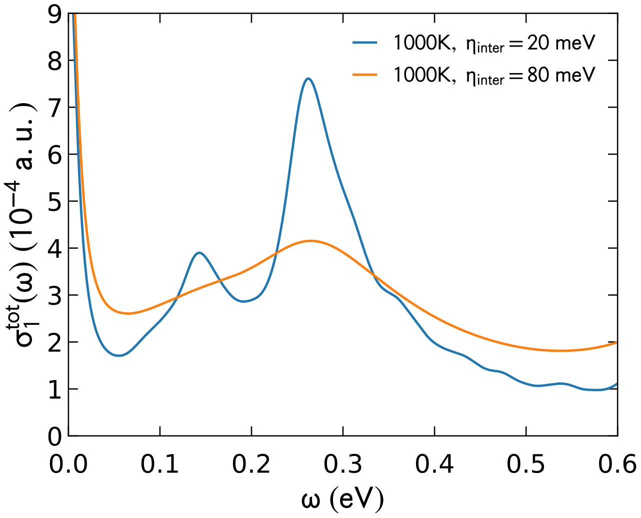


Figure S6: The real part of optical conductivity for the $2 \times 2$ CDW phase at $T = 1000\,\mathrm{K}$, and for low and high value of interband damping parameters $\eta_{\mathrm{inter}}$. The low-energy peak is hardly distinguishable for large $\eta_{\mathrm{inter}}$, which might explain why experimental results for optical conductivity does not report it.

# S3 Comparison between PBE and HSE results

Several theoretical works discussed the importance of going beyond the PBE functional, e.g., by employing the hybrid HSE [S16] or GW approaches, in order to accurately describe the electronic band structure of $TiSe_2$ [S17–S19]. However, so far the corresponding analysis for the optical properties

was not performed.

In Fig. S7 we compare the joint DOS (JDOS), which represents the density of electron-hole pair excitations, as obtained with PBE and HSE functionals. We calculate the JDOS as

$$\mathrm{JDOS}(\omega) = \frac{1}{\omega} \sum_{nm\mathbf{k}} \delta(E_{n\mathbf{k}} - E_{m\mathbf{k}} + \hbar\omega), \tag{S5}$$

which then resembles the optical conductivity formula $\sigma_\mu(\omega)$ as calculated from Eqs. (S1) and (S2). The summations in Eq. (S5) are performed on the momentum grid of $\mathbf{k} = 12 \times 12 \times 1$. By using the PBE calculations, we have checked that this momentum grid is dense enough to accurately represent the positions of the excitation peaks. In Figs. S7(a) and S7(b) we show the results for the low-temperature $2 \times 2$ phase of $TiSe_2$ with distorted atoms when the temperature is far from ($T = 0.09 T_{\mathrm{CDW}}$) and close to the CDW transition ($T = 0.9 T_{\mathrm{CDW}}$). From these results, it is clear that the HSE largely overestimates the energy position of the high-energy (HE) peak [see Fig. S7(c)]. On the other hand, the PBE results are in a good agreement with the experiments [S13,S15], as already shown in Fig. S5 and in the main text. For instance, for $T = 0.09 T_{\mathrm{CDW}}$ the HSE result is $\omega^{\mathrm{HE}} = 0.69$ eV, for the PBE we get $\omega^{\mathrm{HE}} = 0.46$ eV, while the optical conductivity measurments report $\omega^{\mathrm{HE}} = 0.42$ eV. As discussed in the main text, this HE peak comes from the excitations between the highest valence band $v_1$ and second lowest conduction band $c_2$ slightly away from the Brillouin-zone center [as shown in Fig. 1(b) of the main text]. In Fig. S7, we also compare the relative CDW gap modifications obtained with PBE and HSE as a function of temperature. The CDW gap is here defined as the difference between the energies $v_1$ and $c_2$ at the center of the Brillouin zone. The CDW gap results are shown relative to the corresponding values at $T > T_{\mathrm{CDW}}$. Here again the PBE result shows a better agreement with the experiments [S15,S20].

Note that for each of the temperature we relaxed the $2 \times 2$ distorted structures both with PBE and HSE functionals. The obtained PLDs are very similar in both cases, while for the CDW transition temperature we get $T_{\mathrm{CDW}}^{PBE} \approx 1100$ K and $T_{\mathrm{CDW}}^{HSE} \approx 2000$ K, in close agreement with Ref. S18.

Having in mind the good agreement between our PBE results and the optical measurments, as presented in Figs. S5 and S7, as well as in Fig. 3(i) of the main text, we conclude that it is justified

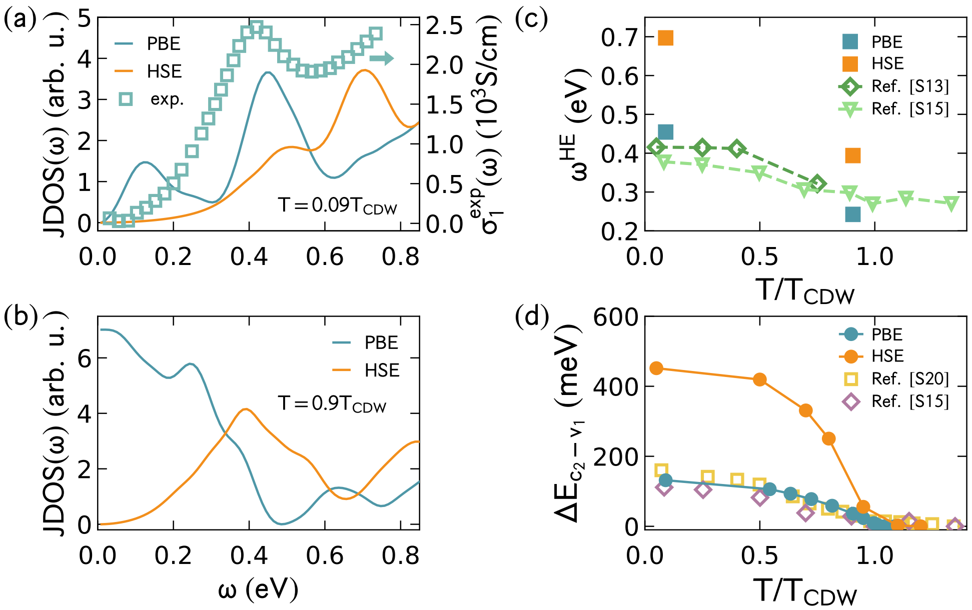


Figure S7: The joint density of states (JDOS) for optical transitions in the distorted $2 \times 2$ phase of $TiSe_2$ monolayer as obtained with PBE (blue) and HSE (orange) functionals when the electronic temperature is (a) far from ($T = 0.09T_{CDW}$) and (b) close to ($T = 0.9T_{CDW}$) the CDW transition. In panel (c) we show the extracted energy positions of the high-energy (HE) peak in JDOS (equivalent to the HE position in the optical conductivity calculations from the main text) as compared to the experiments [S13,S15]. (d) Relative temperature shifts of the CDW gap at the center of the Brillouin zone ($k = \Gamma$) as obtained with the PBE and HSE functionals. The experimental results are from Refs. S15,S20.

to use PBE when simulating the optical properties of $TiSe_2$ across the CDW transition. However, we note that there are several possibilities why the HSE functional fails in reproducing the right position of the HE peak. One is that the excitonic effects are important when the CDW gap is opened, and that the electron-hole attraction if included would reduce the energy of the HE peak [S21]. Another option for $TiSe_2$ would be that the exact exchange in HSE is additionally screened due to a finite concentration of excess charge or due to presence of a substrate (in case of suspended monolayer) [S18].

The phonon-phonon corrections, which were shown to be large in $TiSe_2$ [S18], should not impact the behavior of the optical properties and band gap as a function of temperature. The only difference that we expect in comparison with the present harmonic results would be that the CDW interband peaks and the CDW gap will disappear at the temperatures closer to the experimental value of 200 K.

Further, in Ref. S17 it was shown that the size of the CDW gap is closely related to the strength of the electron-phonon coupling of the CDW-related phonon mode. In fact, it was shown that the CDW gap, and therefore the strength of the electron-phonon coupling, are larger for the HSE functional compared to the PBE. Considering this connection between the CDW gap and strength of the electron-phonon interaction, as well as the good agreement between the PBE and experimental results for the CDW gap and optical properties (but also for PLDs as presented in Fig. S2), one can argue that the PBE results for the electron-phonon scattering rates are close to the actual ones. This might explain the good agreement between the PBE and experimental results for $1/\tau$ in Fig. 2(b) and for the damping rate of the plasmon $\Gamma_{\rm pl}$ in Fig. 3(g) of the main text.

## S4 Optical transitions with spin-orbit coupling

In Fig. S8 we compare the JDOS results with and without the spin-orbit coupling (SOC). The SOC is know to impact the $TiSe_2$ monolayer and bulk, by splitting the degenerate Se-$p$ states around the $\Gamma$ point of the Brillouin zone. However, the impact of the SOC on the phonon dispersions and esimation of the $T_{\rm CDW}$ was shown to be minor [S18]. Here we show in Fig. S8 that SOC has also negligible effects on the optical transitions in the CDW $2\times2$ phase in $TiSe_2$.

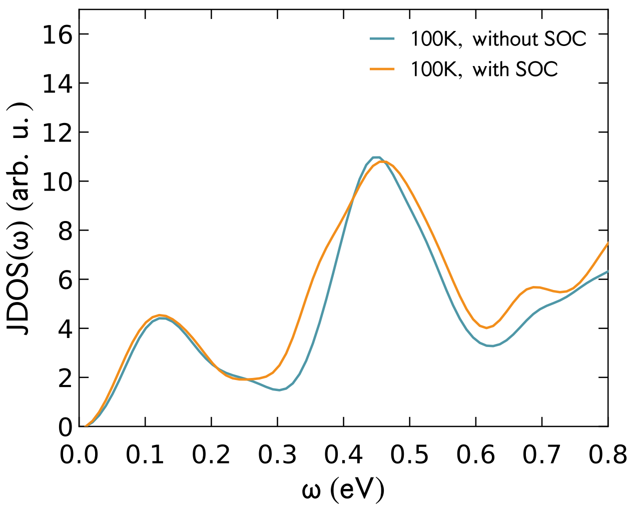


Figure S8: The joint density of states (JDOS) for optical transitions in the distorted $2 \times 2$ phase of $TiSe_2$ monolayer as obtained without (blue) and with (orange) spin-orbit coupling (SOC). The calculations are done with the PBE functional.

## Supporting References


(S1) Giannozzi, P. et al. QUANTUM ESPRESSO: a modular and open-source software project for quantum simulations of materials. *Journal of Physics: Condensed Matter* **2009**, *21*, 395502.

(S2) Hamann, D. R. Optimized norm-conserving Vanderbilt pseudopotentials. *Phys. Rev. B* **2013**, *88*, 085117.

(S3) Perdew, J. P.; Burke, K.; Ernzerhof, M. Generalized Gradient Approximation Made Simple. *Phys. Rev. Lett.* **1996**, *77*, 3865–3868.

(S4) van Setten, M.; Giantomassi, M.; Bousquet, E.; Verstraete, M.; Hamann, D.; Gonze, X.; Rignanese, G.-M. The PseudoDojo: Training and grading a 85 element optimized norm-conserving pseudopotential table. *Computer Physics Communications* **2018**, *226*, 39.

(S5) Mostofi, A. A.; Yates, J. R.; Lee, Y.-S.; Souza, I.; Vanderbilt, D.; Marzari, N. wannier90: A tool for obtaining maximally-localised Wannier functions. *Computer Physics Communications* **2008**, *178*, 685.

(S6) Poncé, S.; Margine, E. R.; Verdi, C.; Giustino, F. EPW: Electron–phonon coupling, transport and superconducting properties using maximally localized Wannier functions. *Computer Physics Communications* **2016**, *209*, 116–133.

(S7) Baroni, S.; de Gironcoli, S.; Dal Corso, A.; Giannozzi, P. Phonons and related crystal properties from density-functional perturbation theory. *Rev. Mod. Phys.* **2001**, *73*, 515.

(S8) Novko, D.; Torbatian, Z.; Lončarić, I. Electron correlations rule the phonon-driven instability in single-layer $TiSe_2$. *Phys. Rev. B* **2022**, *106*, 245108.

(S9) Novko, D.; Šunjić, M.; Despoja, V. Optical absorption and conductivity in quasi-two-dimensional crystals from first principles: Application to graphene. *Physical Review B* **2016**, *93*, 125413.

(S10) Novko, D. Dopant-Induced Plasmon Decay in Graphene. *Nano Letters* **2017**, *17*, 6991.

(S11) Marsiglio, F.; Carbotte, J. P. In *Superconductivity: Conventional and Unconventional Superconductors*; Bennemann, K. H., Ketterson, J. B., Eds.; Springer Berlin Heidelberg: Berlin, Heidelberg, 2008; p 73.

(S12) Fang, X.-Y.; Hong, H.; Chen, P.; Chiang, T.-C. X-ray study of the charge-density-wave transition in single-layer $TiSe_2$. *Phys. Rev. B* **2017**, *95*, 201409.

(S13) Li, G.; Hu, W.; Qian, D.; Hsieh, D.; Hasan, M.; Morosan, E.; Cava, R. J.; Wang, N. Semimetal-to-Semimetal Charge Density Wave Transition in 1 T- TiSe 2. *Physical review letters* **2007**, *99*, 027404.

(S14) Novko, D.; Kralj, M. Phonon-assisted processes in the ultraviolet-transient optical response of graphene. *npj 2D Materials and Applications* **2019**, *3*, 48.

(S15) Monney, C.; Zhou, K. J.; Cercellier, H.; Vydrova, Z.; Garnier, M. G.; Monney, G.; Strocov, V. N.; Berger, H.; Beck, H.; Schmitt, T.; Aebi, P. Mapping of Electron-Hole Excitations

in the Charge-Density-Wave System 1$T$−$TiSe_2$ Using Resonant Inelastic X-Ray Scattering. *Phys. Rev. Lett.* **2012**, *109*, 047401.

(S16) Heyd, J.; Scuseria, G. E.; Ernzerhof, M. Hybrid functionals based on a screened Coulomb potential. *The Journal of Chemical Physics* **2003**, *118*, 8207.

(S17) Hellgren, M.; Baima, J.; Bianco, R.; Calandra, M.; Mauri, F.; Wirtz, L. Critical Role of the Exchange Interaction for the Electronic Structure and Charge-Density-Wave Formation in $TiSe_2$. *Phys. Rev. Lett.* **2017**, *119*, 176401.

(S18) Zhou, J. S.; Monacelli, L.; Bianco, R.; Errea, I.; Mauri, F.; Calandra, M. Anharmonicity and Doping Melt the Charge Density Wave in Single-Layer TiSe2. *Nano Letters* **2020**, *20*, 4809.

(S19) Hellgren, M.; Baguet, L.; Calandra, M.; Mauri, F.; Wirtz, L. Electronic structure of $TiSe_2$ from a quasi-self-consistent $G_0W_0$ approach. *Phys. Rev. B* **2021**, *103*, 075101.

(S20) Monney, C.; Schwier, E. F.; Garnier, M. G.; Mariotti, N.; Didiot, C.; Beck, H.; Aebi, P.; Cercellier, H.; Marcus, J.; Battaglia, C.; Berger, H.; Titov, A. N. Temperature-dependent photoemission on 1$T$-$TiSe_2$: Interpretation within the exciton condensate phase model. *Phys. Rev. B* **2010**, *81*, 155104.

(S21) Mak, K. F.; da Jornada, F. H.; He, K.; Deslippe, J.; Petrone, N.; Hone, J.; Shan, J.; Louie, S. G.; Heinz, T. F. Tuning Many-Body Interactions in Graphene: The Effects of Doping on Excitons and Carrier Lifetimes. *Phys. Rev. Lett.* **2014**, *112*, 207401.
